# Supplementary material for: Automatic Meta-Path Discovery for Effective Graph-Based Recommendation
Source: arXiv:2112.12845 source file (2022-09-07)
Supplement: Supplementary file 1 [file supplement.tex]

\section{Two-level Attention Mechanism}
\label{sec: 2-levelatt}
Figure~\ref{fig:recommender} shows the architecture of two-level attention mechanism and we describe the details here.
\subsection{Node-level Attention}
\label{sec: node-atten}
Note that each meta-path neighbor of a node may have different importance, so we will learn the weight of each meta-path neighbor and aggregate them to form node embeddings before we fuse the information from different meta-paths. Since there are many types of nodes in a HIN, different types of nodes may have different feature spaces. We apply a type-specific projection to project the embeddings of different types of nodes into the same embedding space. The procedure can be formulated as follow:
\vspace{-0.3em}
\begin{equation}
	\label{eq: proj}
	z_i=W_{\phi}x_i,
\end{equation}
where $W_{\phi}$ is the projection matrix of node type $\phi$, $x_i$ and $z_i$ are the original and projected embedding of node $i$ respectively.

After that, suppose nodes $i$ and $j$ are connected via a meta-path $\phi$, the attention score $e^{\phi}_{ij}$ can be calculated using the projected embeddings of nodes $i$ and $j$ by:
\vspace{-0.3em}
\begin{equation}
	\label{eq: n_att}
	e^{\phi}_{ij}=\sigma(\vec a_{\phi}^{T}[z_i | z_j]),
\end{equation}
where $z_i$ and $z_j$ are the projected embeddings of nodes $i$ and $j$ by Equation \ref{eq: proj}, $\vec a_{\phi}$ is the node-level attention vector for meta-path $\phi$, $e^{\phi}_{ij}$ is the attention score of nodes $i$ and $j$ for meta-path $\phi$, $\sigma$ denotes the activation function. Note that the attention score of node $i$ to node $j$ may be different to the attention score of node $j$ to node $i$, which means they may influence each other differently. 

Then for a node $i$, we calculate all the attention score $e_{ij}$ for node  $j \in N^\mathcal{\phi}_{i}$ by Equation \ref{eq: n_att}, where $N^\mathcal{\phi}_{i}$ represents the meta-path neighbors of node $i$ for meta-path $\phi$. After that, we get the importance coefficient $\alpha_{ij}$ by normalizing the attention scores using Softmax~\cite{bridle1990training}:
\vspace{-0.3em}
\begin{displaymath}
	\label{eq: n_norm}
	\alpha_{ij}^{\phi}=\frac{\exp(e_{ij}^{\phi})}{\sum_{k\in N^\mathcal{\phi}_{i}}^{}\exp(e_{ik}^{\phi})}.
\end{displaymath}

Next, we will aggregate neighbor embeddings weighted by the attention scores via the following equation:
\vspace{-0.3em}
\begin{displaymath}
	\label{eq: n_agg}
	h_i^{\phi} =\sigma\left(\sum_{j\in N^\mathcal{\phi}_{i}} {\alpha^{\phi}_{ij} z_j }\right).
\end{displaymath}

Here, $h_i^{\phi}$ is the learned representation of node $i$ for meta-path $\phi$ and $\sigma$ is the activation function. Notice that this attention mechanism can also be extended to multi-head attention~\cite{vaswani2017attention}.

\subsection{Meta-path-level Attention}
\label{sec: meta-atten}

Suppose that we have $X$ meta-paths $\{\phi_1, \dots , \phi_X\}$, after node-level attention, we get $X$ groups of node embeddings, denoted as $\{H_1, \dots , H_X\}$. Since different meta-paths may have different importance for a recommendation task, we propose a meta-path-level attention mechanism to fuse the node embeddings from different meta-paths.

To get the importance of each meta-path, we first transform the embeddings via a multi-layer perceptron (MLP), then multiply with a meta-path-level attention vector $\vec q_{\phi}^T$. Then get the average of all the meta-path-specific node embeddings. The equation is shown as following:
\vspace{-0.3em}
\begin{displaymath}
	\label{eq: m_att}
	w^{\phi_x} =\frac{1}{|\mathcal{V}|}  \sum_{i \in \mathcal{V}}  \vec q_{\phi_x}^{T}  \cdot  \sigma( MLP(h_i^{\phi_x}) ), \  h_i^{\phi_x} \in H_x.
\end{displaymath} 

Here, $\sigma$ is the activation function and $\mathcal{V}$ is the set of all meta-path-specific nodes.

After that, we use softmax function to normalize the meta-path importance as following:
\vspace{-0.3em}
\begin{displaymath}
	\label{eq: m_norm}
	\beta^{\phi_x}=\frac{\exp(w^{\phi_x})}{\sum_{x = 1}^{X}\exp(w^{\phi_x})}.
\end{displaymath}

Here, $\beta^{\phi_x}$ denotes the normalized importance of meta-path $\phi_x$. Lastly, we aggregate the embeddings from each meta-path to get the final node embeddings $H$ according to their weights by:
\vspace{-0.3em}
\begin{displaymath}
	\label{eq: m_agg}
	H =\sum_{x = 1}^{X} \beta^{\phi_x} \cdot H_x.
\end{displaymath}

\section{One-epoch Training Experiment}
\label{sec: sup_one_epoch}
% During the training of the RL agent
To figure out the effectiveness of a meta-path set, we need to use this meta-path set in the recommender training. And during the training, for the efficiency purpose, we only train the recommender for one epoch, then evaluate the performance of the trained model on the evaluation set. To prove this one-epoch training approach is reasonable, we design an experiment on Yelp dataset. We manually designed four meta-path sets.
\begin{itemize}
    \item \textbf{Set1:} UU, BCiB
    \item \textbf{Set2:} UU, UBU, BCiB
    \item \textbf{Set3:} UBU, BUB
    \item \textbf{Set4:} UBU, BUB, BCiB, BCaB
\end{itemize}
% From the results, we found that for most of the cases, if the performance of a model is higher than other models after one-epoch training, its performance will also be better than the other models when the training process converges.
We test each meta-path set in \rec \ algorithm. As shown in Figure~\ref{fig: one-epoch}, we found that even though we only train the model for one-epoch, the effectiveness of Set4 is the best, which is similar when the model converges.

\begin{figure}[]
	\centering
	\includegraphics[width=8.5cm]{./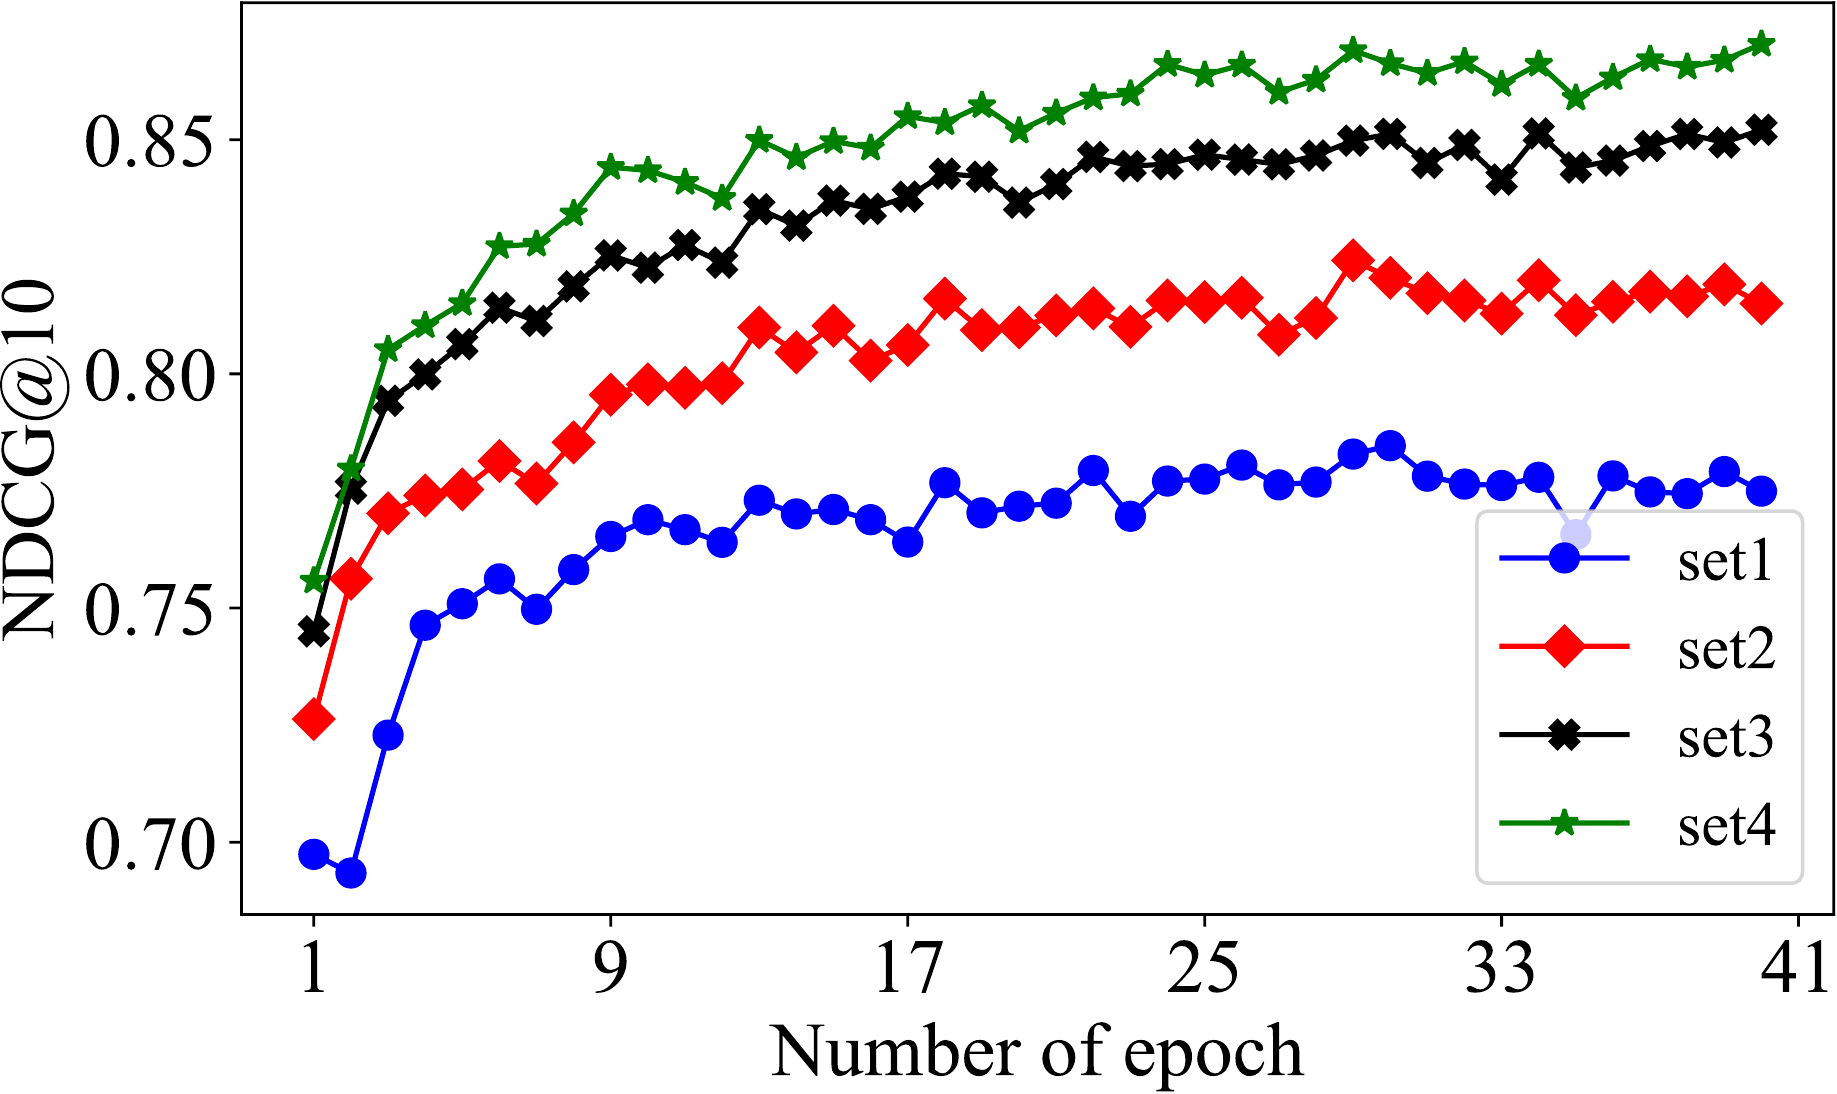}
	\caption{NDCG@10 of each epoch during training}
	\label{fig: one-epoch}
\end{figure}
